# Supplementary material for: Flat2Layout: Flat Representation for Estimating Layout of General Room Types
Source: arXiv:1905.12571 source file (2019-05-29)
Supplement: Supplementary file 2 [file supp_lsun_types.tex]

\section{Definition of LSUN Room Types}
% \begin{figure}[!htb]
% \includegraphics[width=1.8\linewidth]{fig/lsun_types.png}
% \caption{Definition of 11 room types defined in LSUN dataset.}\label{fig:lsun_types}
% \end{figure}
\begin{figure}[!htb]
  \centering
  \setlength\tabcolsep{1pt}
\includegraphics[width=1\linewidth]{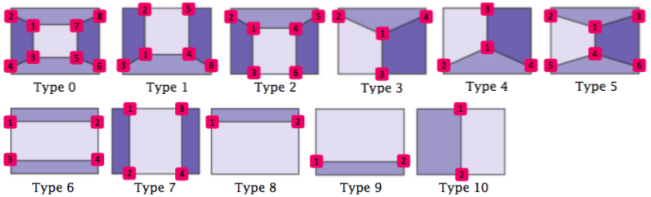}
    \caption{The 11 room types defined in the LSUN dataset.}
    \label{fig:lsun_types}
\end{figure}
